# Supplementary material for: Segment and Caption Anything
Source: arXiv:2312.00869 source file (2024-03-26)
Supplement: Supplementary file 1 [file supp.tex]

\section{Implementation Details}

\cref{sec3:tab:implem_details} presents the implementation details of our method.
Note that as we scale the batch size, the learning rate is scaled linearly as well.
However, during our experiments, we found that there is a maximum threshold of 4e-4.
Scaling the learning rate over 4e-4 leads to underfitting of the data and degradation of performance.
Since we only optimize 19.4M parameters, it costs less computation, less memory usage, and less communication bandwidth, resulting in both fast and scalable training.
We attribute 200K steps of training.
For only VG~\cite{krishnaVisualGenomeConnecting2016a_VG} dataset, we train the models for the full 200K steps.
Otherwise, we first pre-train the models for 100K then finetune them on VG for another 100K steps.
We use 64 V100 GPUs to pre-train and 32 V100 GPUs to finetune.

% Please add the following required packages to your document preamble:
% \usepackage{graphicx}
\begin{table}[t]
\centering
\caption{The implementation details. $\ast$: As the batch size ramps up, the image epoch and region epochs are subjected to be changed, and the learning rate will be scaled linearly \wrt the batch size.}
\label{sec3:tab:implem_details}
{%
\begin{tabular}{l|l}
\toprule
\multicolumn{2}{l}{Optimization}                              \\
\hline
\multirow{2}{*}{Optimizer}    & \multirow{2}{*}{\begin{tabular}[c]{@{}l@{}}AdamW\\ (0.9, 0.999) \\ \hline \end{tabular}}                  \\
                        &                  \\
LR $^\ast$                      & 0.0001                              \\
LR Decay Ratio          & 0                                   \\
LR Decay                & cosine                              \\
Weight Decay            & 0.0001                              \\
Warmup ratio            & 0.3333                              \\
Warmup steps            & 200                                 \\
Gradient Clipping       & 1.0                                 \\
\toprule
\multicolumn{2}{l}{Data Epoch$^\ast$}                                \\
\hline
Batch Size$^\ast$              & 8                                   \\
\# Reg / Img            & 16                                  \\
Steps                   & 200000                              \\
\# Img                  & 77398                               \\
\# Reg                  & 3684063                             \\
Img Epoch$^\ast$               & 20.67                               \\
Reg Epoch$^\ast$               & 6.95                                \\
GPU Type                & V100-16GB                           \\
\# GPUs                 & 8                                   \\
\toprule
\multicolumn{2}{l}{Model Details}                           \\
\hline
\multirow{5}{*}{Input} & \multirow{5}{*}{\begin{tabular}[c]{@{}l@{}} a) 1024x1024\\ Long side: 1024\\ Short side: padding \\b) Large Scale Jitter\\ c) Horizontal Flip \\ \hline \end{tabular}} \\
                        &                  \\
                        &                  \\
                        &                  \\
                        &                  \\
\multirow{2}{*}{Loss}         & \multirow{2}{*}{\begin{tabular}[c]{@{}l@{}} a) Cross Entropy Loss\\ b) Label Smooth (0.1) \\ \hline \end{tabular}} \\
                        &                  \\
\multirow{2}{*}{Text Decoder} & \multirow{2}{*}{\begin{tabular}[c]{@{}l@{}} a) GPT2-large\\ b) Open LLAMA 3B v2 \\ \hline \end{tabular}}       \\
                        &                  \\
\# Query Tokens         & 8                                   \\
\# Mixer Layers         & 12                                  \\
\# Task Tokens          & 6                                   \\
Opt. Module             & Text Feat. Mixer                    \\
\# Opt. Params          & 19.4 M                              \\
\bottomrule
\end{tabular}%
}
\end{table}

\section{Leveraging Other Image Features}

We experiment with image features from other encoders~\cite{radfordLearningTransferableVisual2021b_clip,sunEVACLIPImprovedTraining2023_eva_clip,caronEmergingPropertiesSelfSupervised2021b_dino_facebook,heMaskedAutoencodersAre2021a_mae,darcet2023vitneedreg_dinov2,datacomp2023_datacomp}. 
The training configuration is the same as that of the ablations, which is 8 V100 GPUs and direct decoding when inference.
We use the features from the second last layer~\cite{liu2023improved_llava_1_5}.
We also try to optimize the feature mixer of SAM~\cite{kirillovSegmentAnything2023b_SAM} for the seek of improved performance. The results can be found in~\cref{supp:tab:other_image_encoders}. 
The models with other image encoders perform drastically worse than those with SAM image encoders,
indicating the superiority of the feature space of SAM.
Please note that the image encoders are fixed, other methods like \cite{zhangGPT4RoIInstructionTuning2023a,wangAllSeeingProjectPanoptic2023,wuGRiTGenerativeRegiontotext2022a} need to fine-tune their image encoders,
which increases the computation burden.
While ours only fine-tune the text feature mixer.
It not only achieves better performance but is cheaper for training at scale.

\begin{table}[th]
\centering
\caption{Comparison of using different image encoders. ``C'': CIDEr-D, ``M'': Meteror.}
\label{supp:tab:other_image_encoders}
\begin{tabular}{lcc} 
\toprule
Image
  Encoder                           & {C}             & {M}              \\ 
\hline
vit\_large\_patch14\_clip\_336.openai     & 67.3  & 10.2 \\
vit\_large\_patch14\_clip\_224.datacompxl & 59.0  & 9.3  \\
eva02\_large\_patch14\_clip\_336.merged2b & 53.9  & 8.8  \\
vit\_large\_patch14\_reg4\_dinov2.lvd142m & 76.4  & 11.2 \\
vit\_large\_patch16\_224.mae              & 59.6  & 9.4  \\
\hline
\textit{Add optimization of sam feature mixer}   &         &        \\
vit\_large\_patch14\_clip\_336.openai     & 66.7  & 10.1 \\
vit\_large\_patch14\_clip\_224.datacompxl & 60.3  & 9.5  \\
eva02\_large\_patch14\_clip\_336.merged2b & 54.2  & 8.8  \\
vit\_large\_patch14\_reg4\_dinov2.lvd142m & 76.1  & 11.1 \\
vit\_large\_patch16\_224.mae              & 59.2  & 9.4  \\
\hline
\textit{SAM}                                       & {}                    & {}                    \\
SAM-ViT-base                              & {\cellcolor[rgb]{1,0.851,0.698}}130.2 & {\cellcolor[rgb]{1,0.698,0.698}}16.0  \\
SAM-ViT-large                             & {\cellcolor[rgb]{0.996,1,0.698}}129.6 & {\cellcolor[rgb]{0.996,1,0.698}}15.9  \\
SAM-ViT-huge                              & {\cellcolor[rgb]{1,0.698,0.698}}130.9 & {\cellcolor[rgb]{1,0.851,0.698}}16.0  \\
\bottomrule
\end{tabular}
\end{table}

\section{The results of referring VLLM}

The building of referring Vision Large Language Models (VLLMs) evolves quickly~\cite{wangAllSeeingProjectPanoptic2023,zhangGPT4RoIInstructionTuning2023a}. Here we compare our models with these referring VLLMs in~\cref{supp:tab:comp-ref-vllm}.

\begin{table}[t]
\centering
\caption{
Comparison with referring Vision Large Language Models (VLLMs).
``M'': Meteror, ``C'': CIDEr-D.
$\dagger$: The scores are from the papers. 
$\ddagger$: We reproduced the result with ``GPT4RoI-7B-delta-V0'' from \url{https://github.com/jshilong/GPT4RoI}. 
The best, the second best, the third best scores are marked as \colorbox[rgb]{1,0.698,0.698}{\strut red}, \colorbox[rgb]{1,0.851,0.698}{\strut orange}, \colorbox[rgb]{0.996,1,0.698}{\strut yellow}, respectively.
}
\label{supp:tab:comp-ref-vllm}
\begin{tabular}{lcc} 
\toprule
Method                        & {M}                  & {C}                    \\ 
\hline
ASM~\cite{wangAllSeeingProjectPanoptic2023} (Zero-shot)$^\dagger$                & 12.6                                 & 44.2                                   \\
ASM (Finetuned)$^\dagger$                & {\cellcolor[rgb]{1,0.698,0.698}}18.0 & 145.1                                  \\

GPT4RoI~\cite{zhangGPT4RoIInstructionTuning2023a} (7B)$^\dagger$                   & 17.4                                 & 145.2                                  \\
GPT4RoI (13B)$^\dagger$                 & {\cellcolor[rgb]{1,0.851,0.698}}17.6 & 146.8                                  \\
GPT4RoI (7B)$^\ddagger$                 & 16.4 & 122.3     \\
\hline
SCA (GPT2-large, VG)          & 17.4                                 & {\cellcolor[rgb]{0.996,1,0.698}}148.8  \\
SCA (LLAMA-3B, VG)            & 17.4                                 & {\cellcolor[rgb]{1,0.851,0.698}}149.8  \\
SCA (GPT2-large, Pretrain+VG) & {\cellcolor[rgb]{0.996,1,0.698}}17.5 & {\cellcolor[rgb]{1,0.698,0.698}}149.8  \\
\bottomrule
\end{tabular}
\end{table}

\section{Dataset Statistics}

\cref{tab:exp:data_stats} includes the statistics of the datasets used for training.

\begin{table*}[t]
\centering
\caption{The statistics of region-level understanding datasets used for training. }
\label{tab:exp:data_stats}
\begin{tabular}{l|crrrrr}
\toprule
dataset                          & type        & total samples & total regions & total sents & total tokens & total words \\
\midrule
COCO\cite{linMicrosoftCOCOCommon2015a_mscoco}                   & Region recognition & 117,266       & 860,001       & 860,001     & 1,275,513    & 942,822     \\
V3Det~\cite{wangV3DetVastVocabulary2023a}                     & Region recognition & 183,348       & 1,357,351     & 1,357,351   & 3,984,388    & 2,126,318   \\
Objects365~\cite{shaoObjects365LargeScaleHighQuality2019}                & Region recognition & 1,742,289     & 25,407,598    & 25,407,598  & 49,264,696   & 32,341,116  \\
\midrule
Visual Genome~\cite{krishnaVisualGenomeConnecting2016a_VG} & Region captioning  & 77,398        & 3,684,063     & 3,684,063   & 21,392,494   & 19,740,221  \\
\color{gray} RefCOCOg~\cite{yuModelingContextReferring2016a_refcoco}                  & \color{gray} Referring Expression  & \color{gray} 24,698        & \color{gray} 48,599        & \color{gray} 92,671      & \color{gray} 834,305      & \color{gray} 785,259     \\
\bottomrule
\end{tabular}
\end{table*}

\section{Evaluation of Referring Expression Generation}

Referring Expression Generation (REG)~\cite{yuModelingContextReferring2016a_refcoco,bracha2023disclip} is closely related to regional image captioning.
Regional image captioning is about depicting the regions informatively.
The goal of REG is to output descriptions that discriminate the \textit{unique} object of interest, which does not require faithfully regional descriptions. 
\cref{fig:supp:fig:reg} illustrates the difference with two examples~\cite{bracha2023disclip}.
Despite of the textual style gaps between the two tasks, we present the zero-shot results of REG with our trained models in~\cref{supp:tab:zero-shot-reg}.

\begin{figure}[t]
    \centering
    \includegraphics[width=\linewidth]{figs/diff-img_cap-dense_cap-reg-1.png}
    \includegraphics[width=\linewidth]{figs/diff-img_cap-dense_cap-reg-2.png}
    \caption{The difference between image captioning, regional image captioning, and referring expression generation. The figures are from~\cite{bracha2023disclip}.}
    \label{fig:supp:fig:reg}
\end{figure}

\begin{table*}[t]
\centering

\caption{
The zero-shot performance on the Referring Expression Generation (REG) task. ``M'': Meteror, ``C'': CIDEr-D. 
$\ast$: ``k'' means the number of examples in the prompt.
$\dagger$: The scores are from the papers.
}
\label{supp:tab:zero-shot-reg}
\begin{tabular}{l|cc|cccc|cccc} 
\toprule
\multirow{3}{*}{Method}       & \multicolumn{2}{c|}{RefCOCOg}                                                                        & \multicolumn{4}{c|}{RefCOCO+}                                                                                                                                                                              & \multicolumn{4}{c}{RefCOCO}                                                                                                                                                                                 \\ 
\cline{2-11}
                              & \multicolumn{2}{c|}{val}                                                                             & \multicolumn{2}{c}{testA}                                                                           & \multicolumn{2}{c|}{testB}                                                                           & \multicolumn{2}{c}{testA}                                                                           & \multicolumn{2}{c}{testB}                                                                             \\ 
\cline{2-11}
                              & M             & C                                                    & M             & C                                                    & M             & C                                                    & M             & C                                                    & M             & C                                                      \\ 
\hline
\textit{separate train/test}                                & {}                   &                                                            &                                                            &                                                            &                                                            &                                                            &                                                            &                                                            &                                                              \\
Visdif~\cite{yuModelingContextReferring2016a_refcoco}$^\dagger$                        & 14.5                                 & {-}                  & {14.2}                                 & -                                                          & {13.5}                                 & -                                                          & {18.5}                                 & -                                                          & {{\cellcolor[rgb]{1,0.851,0.698}}24.7} & -                                                            \\
SLR~\cite{yuJointSpeakerListenerReinforcerModel2017a_slr_refcoco}$^\dagger$                           & {\cellcolor[rgb]{1,0.698,0.698}}15.9 & 66.2                                 & {21.3}                                 & {{\cellcolor[rgb]{1,0.698,0.698}}52.0} & {{\cellcolor[rgb]{1,0.698,0.698}}21.5} & {{\cellcolor[rgb]{1,0.698,0.698}}73.5} & {{\cellcolor[rgb]{1,0.698,0.698}}29.6} & {{\cellcolor[rgb]{1,0.698,0.698}}77.5} & {{\cellcolor[rgb]{1,0.698,0.698}}34.0} & {{\cellcolor[rgb]{1,0.698,0.698}}132.0}  \\ 
\hline
\textit{zero-shot}                     & {}                   & {}                   &                                                            &                                                            &                                                            &                                                            &                                                            &                                                            &                                                            &                                                              \\
Kosmos-2~\cite{pengKosmos2GroundingMultimodal2023a}$^\dagger$                      & 12.2                                 & 60.3                                 & -                                                          & -                                                          & -                                                          & -                                                          & -                                                          & -                                                          & -                                                          & -                                                            \\
Kosmos-2 (k=2)$^\ast$$^\dagger$                & 13.8                                 & 62.2                                 & -                                                          & -                                                          & -                                                          & -                                                          & -                                                          & -                                                          & -                                                          & -                                                            \\
Kosmos-2 (k=4)$^\ast$$^\dagger$                 & 14.1                                 & 62.2                                 & -                                                          & -                                                          & -                                                          & -                                                          & -                                                          & -                                                          & -                                                          & -                                                            \\
ASM~\cite{wangAllSeeingProjectPanoptic2023}$^\dagger$                           & 13.6                                 & 41.9                                 & -                                                          & -                                                          & -                                                          & -                                                          & -                                                          & -                                                          & -                                                          & -                                                            \\
GRiT~\cite{wuGRiTGenerativeRegiontotext2022a}                          & 15.2                                 & {\cellcolor[rgb]{0.996,1,0.698}}71.6 & -                                                          & -                                                          & -                                                          & -                                                          & -                                                          & -                                                          & -                                                          & -                                                            \\
SCA (GPT2-large, Pretrain+VG) & {\cellcolor[rgb]{0.996,1,0.698}}15.4 & {\cellcolor[rgb]{1,0.851,0.698}}71.9 & {{\cellcolor[rgb]{0.996,1,0.698}}21.7} & {29.2}                                 & {{\cellcolor[rgb]{1,0.851,0.698}}20.4} & {{\cellcolor[rgb]{1,0.851,0.698}}57.2} & {20.4}                                 & {27.0}                                 & {20.2}                                 & {{\cellcolor[rgb]{0.996,1,0.698}}66.4}   \\
SCA (GPT2-large, VG)          & 15.3                                 & 70.5                                 & {{\cellcolor[rgb]{1,0.851,0.698}}21.7} & {{\cellcolor[rgb]{1,0.851,0.698}}30.2} & {20.1}                                 & {{\cellcolor[rgb]{0.996,1,0.698}}56.6} & {{\cellcolor[rgb]{0.996,1,0.698}}20.5} & {{\cellcolor[rgb]{1,0.851,0.698}}27.7} & {20.1}                                 & {{\cellcolor[rgb]{1,0.851,0.698}}66.7}   \\
SCA (LLAMA-3B, VG)            & {\cellcolor[rgb]{1,0.851,0.698}}15.6 & {\cellcolor[rgb]{1,0.698,0.698}}74.0 & {{\cellcolor[rgb]{1,0.698,0.698}}22.0} & {{\cellcolor[rgb]{0.996,1,0.698}}30.0} & {{\cellcolor[rgb]{0.996,1,0.698}}20.2} & {56.1}                                 & {{\cellcolor[rgb]{1,0.851,0.698}}20.7} & {{\cellcolor[rgb]{0.996,1,0.698}}27.3} & {{\cellcolor[rgb]{0.996,1,0.698}}20.3} & {65.3}                       \\
\bottomrule
\end{tabular}
\end{table*}

\section{Compared with image caption: The distribution of automatic evaluation metrics and the pity of the metrics}
We notice that the convention metrics based on n-gram hold a positive skewness distribution.
Although some predictions perfectly match the ground truths, the overall distribution is still long-tailed.
We plot the distributions of CIDER-D scores for different methods in \cref{sec4:fig:ciderd_dist:sca,sec4:fig:ciderd_dist:sam_cap,sec4:fig:ciderd_dist:grit}.
For ours and GRiT, the distributions are similar.
Whereas more scores are allocated around zero in the SAM-Captioner baseline, leading to poor a average CIDER-D score.
We additionally showcase the distribution of CIDER-D on the image caption dataset COCO in \cref{sec4:fig:ciderd_dist:coco_git}, which is predicted by SOTA image captioner~\cite{wangGITGenerativeImagetotext2022a}
, the distribution is still skewness but is more centered compared with that of region captioning.
For the majority of captions, their CIDER-D score is zero, which does not mean the predictions are wrong, it only indicates there is no n-gram matching.
\eg, The pair ``the windshield of a bus'' and ``large front window on a bus"'' gives zero CIDER-D.
This finding intrigues us to pursue more robust and comprehensive metrics~\cite{kilickaya2016re_metric_re_eval_metrc_image_cap,kornblith2023guiding_metric}.

\input{figs/cider-dist}

\section{Additional Visualizations}

We exhibit more qualitative results in~\cref{sec4:supp:more-vis_infer:1,sec4:supp:more-vis_infer:2}.

\input{figs/supp.comp-qua}

\section{Failure Case Analysis and Limitations}

Our model can make wrong predictions in the terms of following:
\begin{enumerate}
    \item Wrong attribute prediction (\cref{sec4:supp:limitation:wrong-attr}). \eg, the models could predict the wrong colors or textures;
    \item Distinguishing similar visual concepts (\cref{sec4:supp:limitation:wrong-entity}). \eg, the model may confuse ``lemon'' with ``orange'';
    \item Alignment with mask predictions (\cref{sec4:supp:limitation:unalign-mask}): As we do not supervise the alignment, the model may predict mask and captions for the fore- and background separately.
\end{enumerate}

\noindent We believe these drawbacks, \textit{esp.} 1) and 2), may be addressed by weak supervision and self-training~\cite{betkerImprovingImageGeneration_dalle3}.

\input{figs/supp-limitation}
